# Supplementary material for: Potential functionals versus density functionals
Source: arXiv:1307.4235 source file (2013-07-16)
Supplement: Supplementary file 1 [file supp.pdf]

# Supplemental material for "Potential functionals versus density functionals"

Attila Cangi,[1] E.K.U. Gross,[1] and Kieron Burke[2]

[1] *Max Planck Institute of Microstructure Physics, Weinberg 2, 06120 Halle, Germany*[*]

[2] *Department of Chemistry, University of California, Irvine, CA 92697, USA*

(Dated: July 15, 2013)

We provide additional information on the asymptotic analysis to corroborate our conclusions given in Sec. V of the main text. We begin with a global analysis of the total energy in the entire system both in the large-$N$ and the classical continuum limit. Then we repeat the same for distinct spatial regions that correspond to the bulk and surface of a solid. The following analysis is performed for a generic external potential, $v(x) = -8\sin^2 \pi x$ in a box of length 1, assuming that the qualitative results are independent of this particular choice.

We use the following acronyms repeatedly: ISA denotes the independent semiclassical approximation, where two separate semiclassical potential functional approximations (PFA) – both for the density[1] and the kinetic energy density[2] – are used; DSA for the density-driven semiclassical PFA, where only the semiclassical density approximation[1] is used in the coupling-constant construction, first derived in Ref. 3 and studied further in the main text. To avoid repetitions, we refer to material given in the main text (such as equations, tables, and figures) with the following notation: for instance, Eq. (M.$j$) denotes an equation of the main text via the label M, where $j$ corresponds to the equation number.

## I. GLOBAL ANALYSIS

First we investigate the asymptotic behavior of the total energy by expanding it in powers of the particle number $N$. This yields the asymptotic expansion given in Eq. (M.63). We perform an exact calculation and obtain exact coefficients $c_p$. The leading two coefficients $c_0 = \pi^2/6$ and $c_1 = \pi^2/4$ are those of a flat box. We extract the subsequent coefficients numerically by fitting the quantity $(\Delta E + \pi^2/12)/N$ as a function of $1/N$ in the limit $N \to \infty$. The maximum number of particles considered for this numerical analysis is $N = 32$.

Applying the ISA and DSA yields two sets of approximate coefficients, all of which are listed in Tab. I. We evaluate the accuracy of an approximation by its asymptotic exactness (AE$p$), which is defined by the number $p$ of asymptotic coefficients $c_0, c_1, \dots c_p$ an approximation reproduces exactly in the limit $N \to \infty$. Our results demonstrate that the ISA is AE2, because it reproduces all coefficients up to $c_2$ exactly; it is almost AE3, since it approximates $c_3$ very well. However, the DSA has superior accuracy. It reproduces all coefficients up to $c_4$ exactly, making it at least AE4. If we performed a more extensive numerical analysis including larger $N$, also $c_5$ may come out exactly, but this is beyond our computational capabilities. This analysis explains why the DSA is significantly more accurate overall, such as for the total energies listed in Tab. M.I.

TABLE I. Exact and approximate coefficients of the large-$N$ expansion given in Eq. (M.63) for the external potential $v(x) = -8\sin^2(\pi x)$ with $0 \le x \le 1$, where the maximum number of particles considered is $N = 32$.

| | $c_2$ | $c_3$ | $c_4$ | $c_5$ |
|---|---|---|---|---|
| exact | -3.177 | -2.000 | -0.331 | -0.283 |
| ISA | -3.177 | -1.996 | – | – |
| DSA | -3.177 | -2.000 | -0.331 | -0.271 |

Next, we analyze the behavior of the total energy in the classical continuum limit. In Tab. II we report coefficients $b_p$ of the expansion given in Eq. (M.65), as well as the sums of those terms up to the $p$-th order, $E^{(p)}$, for various $N$. The numbers demonstrate the asymptotic nature of Eq. (M.65): For $N = 1$, we see that the result worsens when the third-order contribution is added, and presumably would worsen more with addition of further terms. On the other hand, for $N > 1$, results always improve with addition of terms up to third order. Presumably, one could eventually find a turning point where addition of an extra term worsens the result, but that is beyond our numerical capabilities. We perform the same analyis for the ISA and DSA. Each yields $b_1$ exactly by construction, but they differ in higher-order contributions. In Tab. III we list the absolute error in the coefficients that result from both approximations. The asymptotic nature of the expansion is also apparent in the approximate results. For $N = 1$ the sum up to $p = 3$ of neither the ISA nor DSA converges to the absolute error of the total energies given on the right. As $N$ increases, eventually each additional term improves the result.

We demonstrate this fact further by analyzing how the coefficients in Eq. (M.65) depend on $N$. When we expand in powers of $N$, we obtain

$$b_1 = \frac{\pi^2 N^2}{4L^2}\left(1 + \frac{r_1}{N^2} + \dots\right), \quad (1)$$

where $r_1 = -0.81$ for the present potential, and is given exactly by both approximations. The quadratic coefficient behaves as

$$b_2 = \frac{\pi^2 N}{12L^2}\left(1 + \frac{r_2}{N^4} + \dots\right), \quad (2)$$

* acangi@mpi-halle.mpg.de

TABLE II. Exact coefficients of the classical continuum limit in Eq. (M.65), the sums of that expansion $E^{(p)}$ up to the $p$-th order, and the exact total energy $E$ for a given total particle number $N$ in the external potential $v(x) = -8\sin^2(\pi x)\,,\ 0 \le x \le 1$.

| $N$ | $E^{\mathrm{TF}}$ | $b_1$ | $E^{(1)}$ | $b_2$ | $E^{(2)}$ | $b_3$ | $E^{(3)}$ | $E$ |
|---|---|---|---|---|---|---|---|---|
| 1 | -2.765 | -0.247 | -2.083 | -0.196 | -1.542 | -0.270 | -0.796 | -1.162 |
| 2 | 4.957 | 1.598 | 12.877 | 0.327 | 14.497 | 0.002 | 14.507 | 14.510 |
| 4 | 89.175 | 0.420 | 126.666 | 0.037 | 129.952 | $7{\cdot}10^{-6}$ | 129.953 | 129.953 |
| 8 | 810.156 | 0.193 | 966.073 | 0.008 | 972.652 | 0 | 972.652 | 972.652 |

TABLE III. Performance of the ISA and DSA, where the error is defined as $\Delta b_2^{\mathrm{ISA}} = b_2^{\mathrm{ISA}} - b_2$, etc., for the external potential $v(x) = -8\sin^2(\pi x)\,,\ 0 \le x \le 1$.

| $N$ | $\Delta b_2^{\mathrm{ISA}}$ | $\Delta b_2^{\mathrm{DSA}}$ | $\Delta b_3^{\mathrm{ISA}}$ | $\Delta b_3^{\mathrm{DSA}}$ | $\Delta E^{\mathrm{ISA}}$ | $\Delta E^{\mathrm{DSA}}$ |
|---|---|---|---|---|---|---|
| 1 | 0.052 | -0.042 | 0.038 | 0.140 | -0.183 | -0.022 |
| 2 | 0.002 | 0.003 | -0.036 | -0.002 | -0.120 | 0.005 |
| 4 | $-10^{-5}$ | $-2{\cdot}10^{-5}$ | $-5{\cdot}10^{-4}$ | $-10^{-5}$ | -0.036 | 0.001 |
| 8 | 0 | 0 | $-10^{-5}$ | 0 | -0.01 | $2{\cdot}10^{-4}$ |

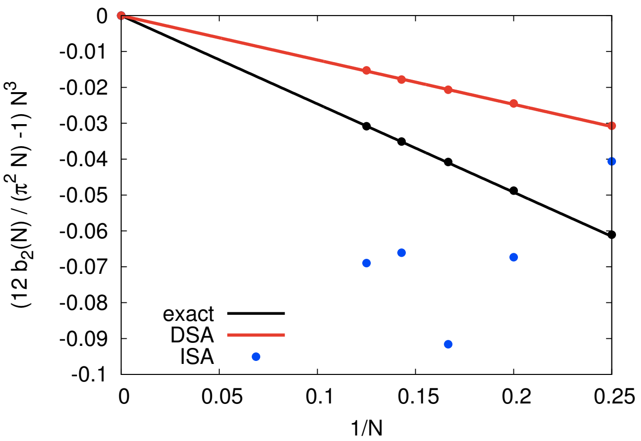


FIG. 1. Exact (black) coefficients $b_2$ of the classical continuum limit in Eq. (M.65) in comparison to the DSA (red) and ISA (blue) as a function of the particle number $N$ for $v(x) = -8\sin^2(\pi x)\,,\ 0 \le x \le 1$.

which is shown in Fig. 1. The exact coefficient is $r_2 = -0.24$, the DSA yields a value $r_2^{\mathrm{DSA}} = -0.12$, which is half as big. But the ISA does not yield a well-defined $N$-dependence of this coefficient, which explains its inaccuracy for small $N$.

## II. LOCAL ANALYSIS: SURFACE VS. BULK

We repeat the asymptotic analysis both in the large-$N$ and the classical continuum limit, but now focusing on contributions from the interior and the region close to the edge. We choose the half-phase point, $x_{\pi/2}$, defined by Eq. (M.67) as the boundary between those two characteristic regions. In both limits, i.e., as $N$ increases, the relative size of both regions changes; the size of the edge region shrinks, whereas the interior grows. Therefore the leading coefficient of either expansion in the region close to the edge does not contribute, i.e., $c_0^{\mathrm{edge}} = 0$ and $b_0^{\mathrm{edge}} = 0$. Also note that we need to distinguish between two exact energies when we divide up space into separate regions. This is due to the fact that we use two different definitions of the kinetic energy density. The first corresponds to the Laplacian definition and is used in the ISA. The other definition for the DSA is due to the functional integration via the coupling-constant method. The difference of those definitions is illustrated in Fig. (M.4).

TABLE IV. Exact and approximate asymptotic coefficients in the interior ($c_p^{\mathrm{int}}$) and the edge region ($c_p^{\mathrm{edge}}$) for the external potential $v(x) = -8\sin^2(\pi x)$ with $0 \le x \le 1$, where the maximum number of particles considered is $N = 24$.

| | interior | | | edge | | |
|---|---|---|---|---|---|---|
| | $c_1$ | $c_2$ | $c_3$ | $c_1$ | $c_2$ | $c_3$ |
| exact | 1.31 | -4.29 | -0.410 | 1.15 | 0.93 | 1.593 |
| exact (cc) | 1.32 | -4.56 | -0.406 | 1.14 | 1.23 | 0.059 |
| ISA | 1.31 | -4.29 | -0.413 | 1.15 | 0.93 | 1.595 |
| DSA | 1.32 | -4.56 | -0.406 | 1.14 | 1.23 | 0.059 |

We begin with the large-$N$ expansion of the total energy. The energy in the interior and close to the edge can be expanded in analogy to Eq. (M.63), with coefficients $c_p^{\mathrm{int}}$ and $c_p^{\mathrm{edge}}$. The numerical values of the coeffcients up to the third order are listed in Tab. IV. We could not perform the numerical analysis at higher orders reliably; this is due to the division of space which causes minuscule oscillations in the total energy attributed to each region, whose effect gets magnified for higher order coefficients. Nevertheless, the results in Tab. IV agree with our global analysis. Both in the interior and close to the edge the ISA reproduces the first two coefficients exactly, making it AE2. The DSA is more accurate – at least AE3 – because it is capable of yielding coefficients up to the third order exactly and likely also beyond that order, but confirming this is beyond our numerical capabilities.

Next we analyze the behavior of total energy in each region while approaching the classical continuum limit, i.e., when $\gamma \to 0$. In Tab. V we list the exact quantities, such as the coefficients $b_p$ up to the second order, $E^{(p)}$, and the total energy in the interior and close to the edge for various $N$. The asymptotic nature of that expan-

TABLE V. Exact coefficients of the classical continuum limit in Eq. (M.65) for the interior and close to the edge, the sums of that expansion $E^{(p)}$ up to the $p$-th order, and the exact total energy $E$ as a function of the total particle number $N$ in the external potential $v(x) = -8\sin^2(\pi x)\,,\ 0 \leq x \leq 1$.

| | interior | | | | | | edge | | | | | |
|---|---|---|---|---|---|---|---|---|---|---|---|---|
| $N$ | $E^{\rm TF}$ | $b_1$ | $E^{(1)}$ | $b_2$ | $E^{(2)}$ | $E$ | $E^{\rm TF}$ | $b_1$ | $E^{(1)}$ | $b_2$ | $E^{(2)}$ | $E$ |
| 1 | -2.76 | -0.11 | -2.45 | -0.538 | -0.96 | -0.67 | – | -0.13 | 0.37 | 0.247 | -0.32 | -0.49 |
| 2 | 4.96 | 0.84 | 9.12 | 0.010 | 9.17 | 9.63 | – | 0.75 | 3.70 | 0.351 | 5.44 | 4.87 |
| 4 | 89.18 | 0.22 | 109.05 | -0.007 | 108.39 | 108.55 | – | 0.20 | 17.38 | 0.048 | 21.62 | 21.35 |
| 8 | 810.16 | 0.10 | 893.04 | -0.002 | 891.25 | 891.23 | – | 0.09 | 72.10 | 0.011 | 80.85 | 81.03 |

TABLE VI. Performance of the ISA and DSA in the interior and close to the edge for the external potential $v(x) = -8\sin^2(\pi x)\,,\ 0 \leq x \leq 1$.

| | interior | | | | edge | | | |
|---|---|---|---|---|---|---|---|---|
| $N$ | $\Delta b_2^{\rm ISA}$ | $\Delta b_2^{\rm DSA}$ | $\Delta E^{\rm ISA}$ | $\Delta E^{\rm DSA}$ | $\Delta b_2^{\rm ISA}$ | $\Delta b_2^{\rm DSA}$ | $\Delta E^{\rm ISA}$ | $\Delta E^{\rm DSA}$ |
| 1 | 0.01 | 0.11 | -0.10 | -0.08 | 0.35 | -0.03 | -0.02 | -0.02 |
| 2 | -0.12 | 0.06 | -0.15 | 0.03 | 0.01 | $-10^{-4}$ | 0.01 | $-10^{-3}$ |
| 4 | -0.06 | 0.03 | -0.07 | 0.03 | $10^{-3}$ | 0 | $10^{-3}$ | $-10^{-4}$ |
| 8 | -0.03 | 0.01 | -0.02 | 0.01 | $2{\cdot}10^{-4}$ | 0 | $2{\cdot}10^{-4}$ | 0 |

sion is apparent; for example, in the interior $E^{(2)}$ seems to be converging to the total energy with increasing $N$, but for $N = 8$ the coefficient $b_2^{\rm int}$ is already overcorrecting. By construction both the ISA and DSA yield the correct leading correction to the total energy as the classical continuum limit is approached. This is also the case when we consider the distinct energy contributions coming from the interior and the region close to the edge. To complement the conclusion given in the main text we report the numerical results assessing the performance of the ISA and DSA in Tab. VI.


[1] P. Elliott, D. Lee, A. Cangi, and K. Burke, Phys. Rev. Lett. **100**, 256406 (2008).

[2] A. Cangi, D. Lee, P. Elliott, and K. Burke, Phys. Rev. B **81**, 235128 (2010).

[3] A. Cangi, D. Lee, P. Elliott, K. Burke, and E. K. U. Gross, Phys. Rev. Lett. **106**, 236404 (2011).
